# Supplementary material for: Reference-Free Isotropic 3D EM Reconstruction using Diffusion Models
Source: arXiv:2308.01594 source file (2023-08-03)
Supplement: Supplementary file 1 [file 6_supplement.tex]

\setcounter{table}{0}

\setcounter{figure}{0}

\begin{figure}[t]%[h]
    \centering
    \includegraphics[width=0.99\textwidth]{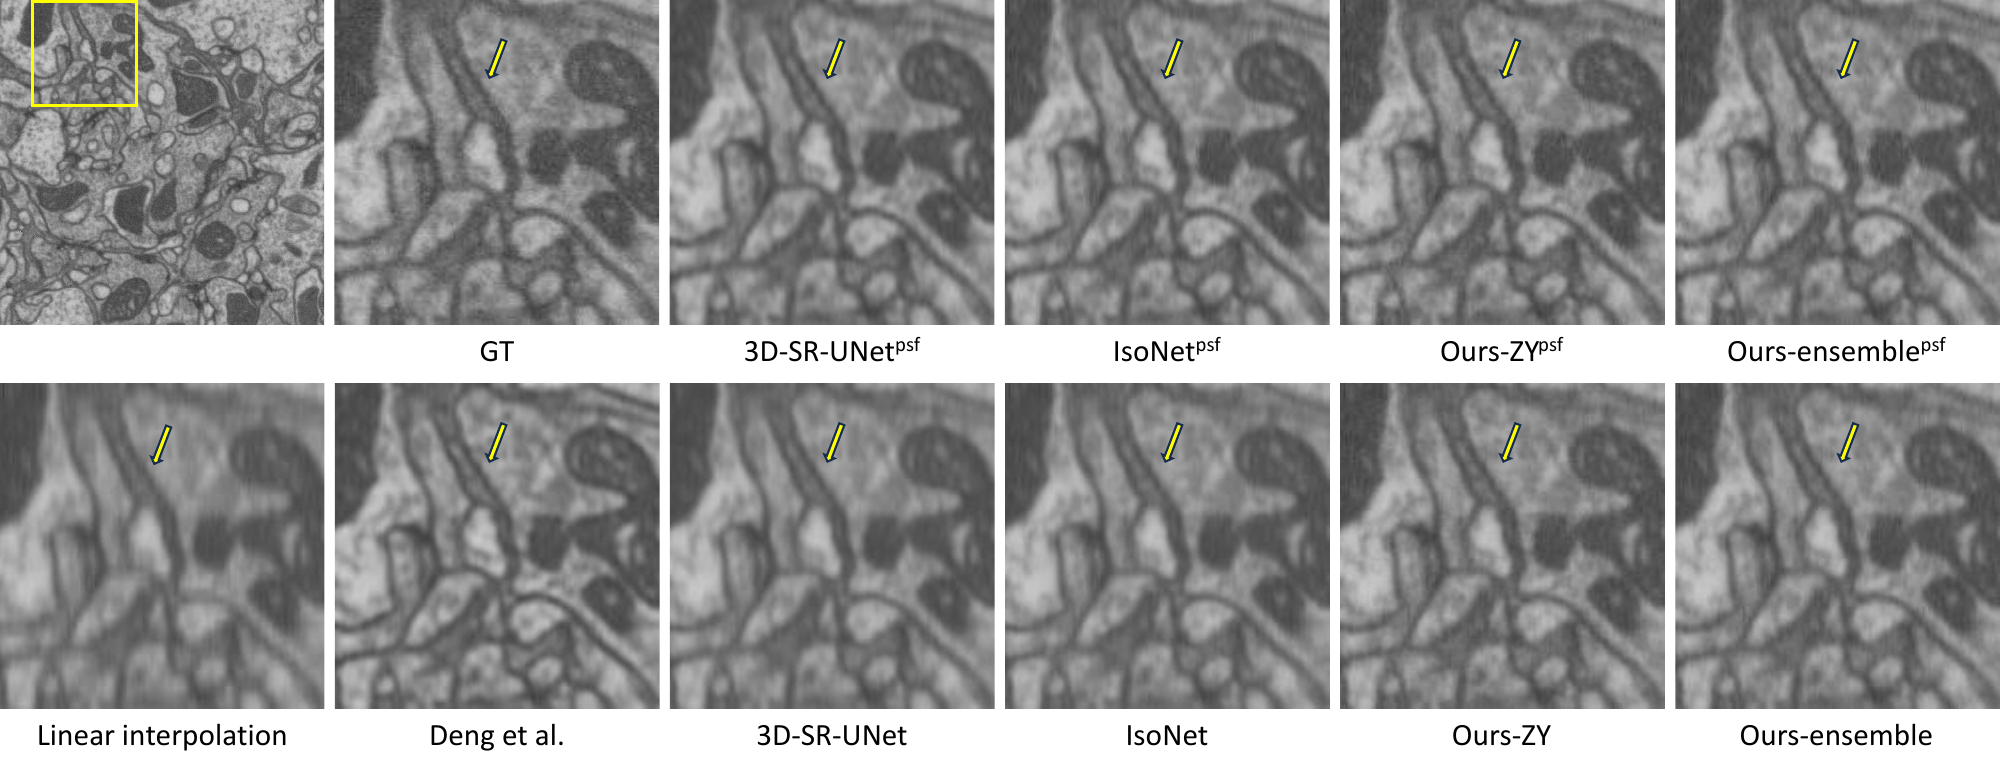}
    \caption{
    Qualitative comparison of FIB25 reconstruction viewed in ZY. With $f=4$ and a Gaussian filter of $\sigma=2$, the isotropic FIB25 volume is simulated to an anisotropic resolution of $128\times512\times512$.
    Superscript PSF indicates that the exact point spread function was used for reconstruction.
    }
    \label{figure:fib25_factor4}
\end{figure}

\begin{table}[tb]%[htb!]
\centering
\caption{Quantitative Comparison with other methods. With $f=4$ and a Gaussian filter of $\sigma=2$, the isotropic FIB25 volume is simulated to an anisotropic resolution of $128\times512\times512$. The baseline is linear interpolation. $\perp$ and $+$ indicate that the reconstruction was done on ZX slices or is ensembled, respectively. The highest scores are highlighted in \textbf{bold}.}
\label{table:fib25_factor4}

\setlength{\tabcolsep}{0.3pt}
\scriptsize{
\begin{tabular}{|c|c|ccc|ccc|ccc|}
\hline
\multirow{3}{*}{\textbf{PSF}} & \multirow{2}{*}{\textbf{Method}} & \multicolumn{3}{|c|}{\textbf{ZY}}  &\multicolumn{3}{|c|}{\textbf{ZX}} & \multicolumn{3}{|c|}{\textbf{XY}} \\
& & PSNR$\uparrow$ & MS-SSIM$\uparrow$ & LPIPS$\downarrow$ & PSNR$\uparrow$ & MS-SSIM$\uparrow$ & LPIPS$\downarrow$ & PSNR$\uparrow$ & MS-SSIM$\uparrow$ & LPIPS$\downarrow$ \\
\cline{2-11}
& Baseline & 29.50 & 0.944 & 0.438 & 29.51 & 0.943 & 0.432 & 29.58 & 0.938 & 0.280 \\
\cline{1-11}

\multirow{4}{*}{Exact} & 3D-SR-UNet & 31.94 & 0.979 & 0.422 & 31.97 & 0.976 & 0.418 & 32.01 & 0.973 &0.338\\
\cline{2-11}
& IsoNet & \textbf{32.44} & \textbf{0.982} & 0.406 & \textbf{32.48} & \textbf{0.981} & 0.402 & \textbf{32.57} & \textbf{0.975} & 0.203\\
\cline{2-11}
& Ours & 31.65 & 0.978 & \textbf{0.262} & 31.67 & 0.978 & \textbf{0.279} & 31.76 & 0.971 & 0.181\\
\cline{2-11}
& Ours\textsuperscript{$+$} & 32.11 & 0.981 & 0.325 & 32.14 & 0.979 & 0.321 & 32.23 & 0.973 & \textbf{0.175}\\
\hline

\multirow{6}{*}{Blind} & 3D-SR-UNet & 30.57 & 0.963 & 0.431 & 30.59 & 0.961 & 0.426 & 30.62 & 0.958 &0.368\\
\cline{2-11}
& IsoNet & 30.84 & 0.966 & 0.409 & 30.86 & 0.964 & 0.405 & 30.91 & 0.959 & 0.254\\
\cline{2-11}
& Deng \textit{et al.} & 30.26 & 0.967 & 0.444 & 30.27 & 0.965 & 0.427 & 30.31 & 0.961 & 0.350\\
\cline{2-11}
& Ours & 30.87 & 0.970 & \textbf{0.266} & 30.89 & 0.969 & 0.288 & 30.96 & 0.962 & 0.205 \\
\cline{2-11}
& Ours\textsuperscript{$\perp$} & 30.91 & 0.971 & 0.292 & 30.93 & 0.969 & \textbf{0.275} & 31.00 & 0.963 & \textbf{0.189} \\
\cline{2-11}
& Ours\textsuperscript{$+$} & \textbf{31.22} & \textbf{0.972} & 0.326 & \textbf{31.24} & \textbf{0.971} & 0.324 & \textbf{31.30} & \textbf{0.965} & 0.199\\
\hline
\end{tabular}
}
\end{table}

\clearpage

\begin{figure}[th]%[h]
    \centering
    \includegraphics[width=1.02\textwidth]{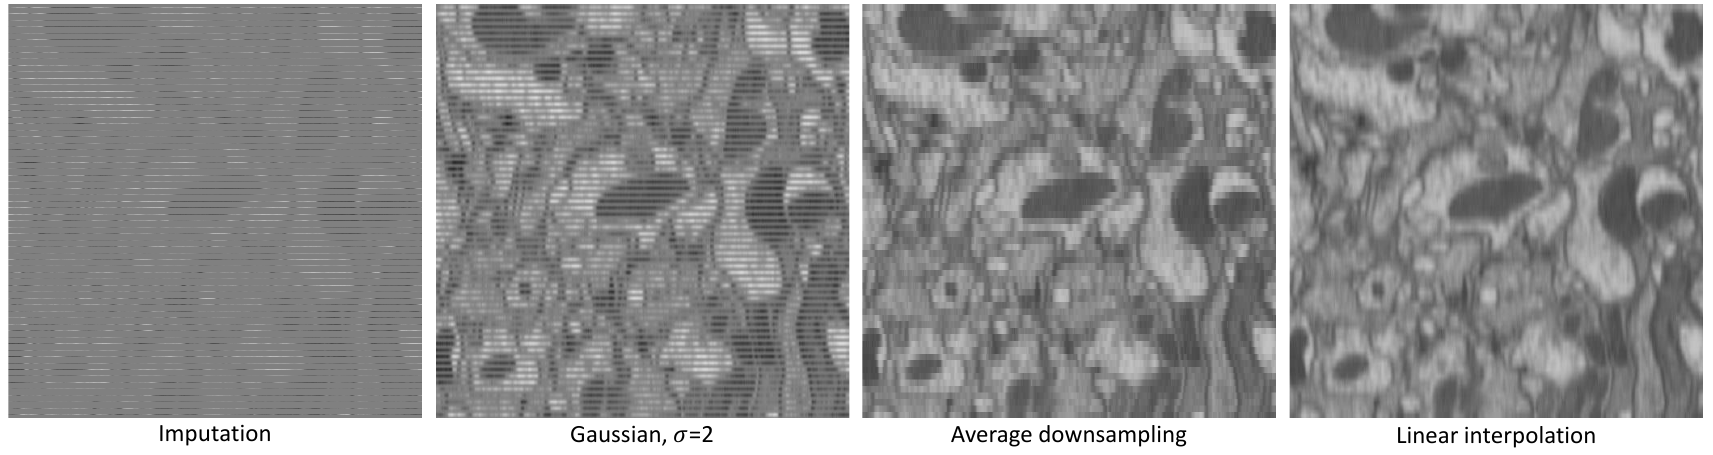}
    \caption{
    Visaulization of $\textbf{A}^\dagger\textbf{y}$ given various degradation assumptions. The data was simulated with $\sigma=2, f=8$. From left to right: Imputation, Gaussian filter of $\sigma=2$, average downsampling and linear downsampling, respectively.
    The diffusion model fills in the missing high-frequency components to realistically reconstruct the anisotropic axial slices. As shown, starting the reconstruction from linear interpolation lightens the burden compared to imputation or wrong gaussian kernel.
    }
    \label{figure:degradation}
\end{figure}

\begin{table}[htb!]
\caption{Abalation for assumption of the degradation. The highest scores are highlighted in \textbf{bold}.}
\centering
\label{table:ablation_A}

\setlength{\tabcolsep}{4.0pt}
\scriptsize{
\begin{tabular}{|c|ccc|}
\hline
\textbf{Method} & PSNR$\uparrow$ & MS-SSIM$\uparrow$  & LPIPS$\downarrow$ \\
\hline
Imputation& 25.06 & 0.802 & 0.495\\
\cline{1-4}
Gaussian, $\sigma=2$& 26.82 & 0.873 & 0.418\\
\cline{1-4}
Average& 26.91 & 0.878 & 0.415\\
\cline{1-4}
Interpolation& \textbf{27.55}& \textbf{0.901} & \textbf{0.391}\\
\hline
\end{tabular}
}
\end{table}

%\scriptsize{
%\begin{tabular}{|c|ccc|}
%\hline
%\textbf{method} & PSNR & MS-SSIM  & LPIPS \\
%\hline
%inpaint& 25.06 & 0.802 & 0.495\\
%\cline{1-4}
%gau $\sigma=2$& 26.82 & 0.873 & 0.418\\
%\cline{1-4}
%average& 26.91 & 0.878 & 0.415\\
%\cline{1-4}
%Ours& 27.55& 0.901 & 0.391\\
%\hline
%\end{tabular}
%}
